# Supplementary material for: On the Predictive Risk in Misspecified Quantile Regression
Source: arXiv:1802.00555 source file (2018-11-01)
Supplement: Supplementary file 1 [file PredRiskQR_Supplement_v3-arXiv.pdf]

# Supplementary Materials for “On the Predictive Risk in Misspecified Quantile Regression”

## S.1. On the interpretation of misspecified quantile regression

Our setting of persistently misspecified quantile regression models as outlined in Section 2.1 generalizes the framework of Angrist et al. (2006) to the case in which the number of predictors grows with the sample size. Angrist et al. (2006) (Theorem 1) show that the solution to the quantile regression problem (4) under persistent misspecification can be interpreted as the best linear approximation to the true CQF under a weighted square loss with (random) weights that down weight regions of the parameter space in which the conditional density of  $Y_{n1}$  given  $X_{n1}$ ,  $f_{Y_n|X_n}$ , is low, i.e.  $\theta_{n,S}^\tau$  equivalently solves

$$\min_{\theta \in \mathbb{R}^{|S|}} \mathbb{E}_{\mathcal{D}_n} \left[ \omega^\tau \cdot \left( Q_{Y_n}(\tau|X_{n1}) - Z_S(X_{n1})'\theta \right)^2 \right], \quad (\text{S.1.1})$$

where

$$\omega^\tau \equiv \omega^\tau(X_{n1}, S) = \int_0^1 (1-u) f_{Y_n|X_n} \left( u \cdot Z_S(X_{n1})'\theta + (1-u) \cdot Q_{Y_n}(\tau|X_{n1}) | X_{n1} \right) du.$$

As an immediate consequence of this result we have the following relation between the predictive risk based on the check loss  $\rho_\tau$  and the (weighted) mean squared prediction error.

**Proposition S.1.1.** *Suppose that  $\mathbb{E}_{X_n^0} [Q_{Y_n^0}(\tau|X_n^0)]$  is finite and  $\theta_{n,S}^\tau$  uniquely solves (4). Then, the predictive risk satisfies*

$$\text{PR}_n^\tau(S) = \mathbb{E}_{\mathcal{D}_n, X_n^0} \left[ \omega^\tau(\mathcal{D}_n, X_n^0, S) \cdot \left( Q_{Y_n^0}(\tau|X_n^0) - \widehat{Q}_{Y_n^0}(\tau|X_n^0, S) \right)^2 \right] + \left( \mathbb{E}_{X_n^0} [F_{Y_n^0|X_n^0}(0|X_n^0)] - \tau \right). \quad (\text{S.1.2})$$

where

$$\omega^\tau(\mathcal{D}_n, X_n^0, S) = \int_0^1 (1-u) f_{Y_n^0|X_n^0} \left( u \cdot \widehat{Q}_{Y_n^0}(\tau|X_n^0, S) + (1-u) \cdot Q_{Y_n^0}(\tau|X_n^0) | X_n^0 \right) du.$$

*Proof.* Add and subtract  $\widehat{Q}_{Y_n^0}(\tau|X_n^0, S)$  in expression S.1.1 and expand the squares.  $\square$

Note that the second term on the right in eq. (S.1.2) is a constant in the interval  $(-\tau, 1-\tau)$  and independent of sample  $\mathcal{D}_n$ , quantile model  $S$ , and estimate  $\widehat{Q}_{Y_n^0}(\tau|X_n^0, S)$ ; only the first term depends on the data and the model. This first term is a weighted version of the mean squared prediction error with weights that down-weight regions on the real line where the conditional density of  $Y_n^0$  given  $X_n^0$  is low. Angrist et al. (2006) demonstrate that for most practical purposes the weight  $\omega^\tau$  tends to be constant across  $X_n^0$ . Thus, we can think of the predictive risk  $\text{PR}_n^\tau(S)$  as a nearly affine transformation of the mean squared prediction error  $\mathbb{E}_{\mathcal{D}_n, X_n^0} [(Q_{Y_n^0}(\tau|X_n^0) - \widehat{Q}_{Y_n^0}(\tau|X_n^0, S))^2]$ .

## S.2. On model selection via the de-biased predictive risk estimate

Our de-biased, uniformly consistent, estimate of the predictive risk from Section 4.2 can be used to construct an Akaike-type information criterion which satisfies a notion of model selection consistency even if the regression model is misspecified.

The principal idea underlying Akaike-type information criteria is to choose a model  $S$  that minimizes the expected Kullback-Leibler divergence between the density associated with target  $\mu$  and the density associated with estimate  $\hat{\mu}_{n,S}$  (e.g. [Lv and Liu, 2014](#); [Akaike, 1992, 1998](#)). For general  $M$ -estimators, whose minimizers are not associated with a density, this approach amounts to choosing a model  $S$  that minimizes the expected predictive risk associated with the estimate  $\hat{\mu}_{n,S}$ . More precisely, we define the model with minimum predictive risk,  $S_n^*$ , and its sample analogue,  $\hat{S}_n$ , as

$$S_n^* = \arg \min_{S \in M} \text{PR}_n^\tau(S) \quad \text{and} \quad \hat{S}_n = \arg \min_{S \in M} \widehat{PR}_{n,h}^\tau(S). \quad (\text{S.2.1})$$

We have the following result.

**Proposition S.2.1** (Model Selection Consistency for Minimum Predictive Risk Model). *Suppose that the conditions of Corollary 3 hold and that  $S_n^*$  is the unique minimizer of  $\text{PR}_n^\tau$ . If  $n^{1/4}h \sim (m \log |M| \log \log n)^{1/4}$ , then  $\lim_{n \rightarrow \infty} \mathbb{P}(\hat{S}_n = S_n^*) = 1$ .*

*Proof.* By the optimality of  $S_n^*$  and  $\hat{S}_n$  we have

$$\begin{aligned} 0 &\leq \text{PR}_n^\tau(\hat{S}_n) - \text{PR}_n^\tau(S_n^*) = \text{PR}_n^\tau(\hat{S}_n) - \widehat{PR}_{n,h}^\tau(\hat{S}_n) + \widehat{PR}_{n,h}^\tau(\hat{S}_n) - \text{PR}_n^\tau(S_n^*) \\ &\leq \text{PR}_n^\tau(\hat{S}_n) - \widehat{PR}_{n,h}^\tau(\hat{S}_n) + \widehat{PR}_{n,h}^\tau(S_n^*) - \text{PR}_n^\tau(S_n^*) \\ &\leq 2 \sup_{S \in M} \left| \text{PR}_n^\tau(S) - \widehat{PR}_{n,h}^\tau(S) \right| \rightarrow 0, \end{aligned}$$

where the last inequality follows from Theorem 4. The claim follows since by assumption  $S_n^*$  is unique.  $\square$

This proposition states that, under weak conditions and arbitrary misspecification, the minimizer of the de-biased predictive risk estimate,  $\hat{S}_n$ , is consistent for the (population) minimum predictive risk model,  $S_n^*$ . If the true model  $S_0$  is contained in the family of candidate models  $M$ , then it holds that  $S_n^* = S_0$ . Thus, in this case, model selection based on the de-biased predictive risk estimate is model selection consistent in the traditional sense, i.e. for  $S_0$ .

## S.3. Technical lemmata

**Lemma S.3.1** ([Panchenko \(2003\)](#)). *Let  $X_1, \dots, X_n, X_1^0, \dots, X_n^0$  be i.i.d. random vectors on a measurable space  $\mathcal{X}$  and let  $\mathcal{F} = \{f : \mathcal{X} \rightarrow \mathbb{R}\}$  be a countable class of measurable functions. Define*

the mixed uniform variance as

$$V = \mathbb{E}_{X^0} \left[ \sup_{f \in \mathcal{F}} \sum_{i=1}^n (f(X_i) - f(X_i^0))^2 \right].$$

Then for any  $\alpha > 0$  and  $t > 0$ ,

$$\mathbb{P} \left( \sup_{f \in \mathcal{F}} \sum_{i=1}^n f(X_i) \geq \mathbb{E}_X \left[ \sup_{f \in \mathcal{F}} \sum_{i=1}^n f(X_i) \right] + 2\sqrt{Vt} \right) \leq 2^{\alpha+1} \exp \left\{ 1 - \frac{\alpha}{\alpha+1} t \right\}$$

and

$$\mathbb{P} \left( \sup_{f \in \mathcal{F}} \sum_{i=1}^n f(X_i) \leq \mathbb{E}_X \left[ \sup_{f \in \mathcal{F}} \sum_{i=1}^n f(X_i) \right] - 2\sqrt{Vt} \right) \leq 2^{\alpha+1} \exp \left\{ 1 - \frac{\alpha}{\alpha+1} t \right\}.$$

The next two technical lemmata are needed in the consistency proofs involving the matrices  $D_{n,0}^\tau(S)$  and  $D_{n,1}^\tau(S)$ .

**Lemma S.3.2.** *Let  $\{(W_n, X_n), (W_{ni}, X_{ni}), i = 1, \dots, n\}$  be a triangular array of row-wise i.i.d. random vectors in  $\mathbb{R} \times \mathbb{R}^d$ . Suppose that  $W_n|X_n$  has a continuous distribution function and density bounded by  $F_+ > 0$ . Let  $g : \mathbb{R}^d \rightarrow \mathbb{R}$  be an arbitrary function with envelope  $G$  such that  $\mathbb{E}[G^{4+2\delta}] < \infty$  for some  $\delta > 0$ . Then, for all  $r_n > 0$  there exists an absolute constant  $c_0 > 0$  such that*

$$\begin{aligned} & \mathbb{E}_{W,X} \left[ \sup_{\|\theta\|_2=r_n} \frac{1}{n} \sum_{i=1}^n \left( 1 \{0 < W_{ni} \leq X'_{ni}\theta\} g(X_{ni}) - \mathbb{E}_{W,X} [1 \{0 < W_{ni} \leq X'_{ni}\theta\} g(X_{ni})] \right) \right] \\ & \leq c_0 \left( \frac{d}{n} \right)^{3/4} \mathbb{E}[G^4(X_{n1})]^{1/4} \mathbb{E}[G^{4+2\delta}(X_{n1})]^{1/(4+2\delta)} \mathbb{E}[G^{2+\delta}(X_{n1})]^{1/(2+\delta)} \\ & \quad + c_0 r_n^{1/2} \left( \frac{d}{n} \right)^{1/2} F_+^{1/2} \sup_{\|u\|_2=1} \mathbb{E}[(X'_{n1}u)G^2(X_{n1})]^{1/2} \mathbb{E}[G^{2+\delta}(X_{n1})]^{1/(2+\delta)}. \end{aligned}$$

*Proof.* We combine a combinatorial (i.e. sample distribution independent) bound on the entropy of a conditional Rademacher average with a probabilistic (i.e. sample distribution dependent) bound on the second and fourth moments of the corresponding unconditional Rademacher average. This allows us to leverage the fact that the variance of the unconditional Rademacher process is proportional to  $r_n$ .

**Step 1. VC-index and covering numbers.** For  $r_n > 0$  and a function  $g : \mathbb{R}^d \rightarrow \mathbb{R}$  with envelop  $G$  define the class of functions

$$\mathcal{F}(r_n) = \left\{ (W, X) \mapsto 1 \{0 < W \leq X'\theta\} g(X) : \|\theta\|_2 \leq r_n, \theta \in \mathbb{R}^d \right\}.$$

Without loss of generality we can assume that  $G \geq 1$ . Define

$$\tilde{\mathcal{F}}(r_n) = \{f/G : f \in \mathcal{F}(r_n)\}.$$

Denote by  $\Gamma$  the collection of subgraphs of  $f \in \tilde{\mathcal{F}}(\infty)$ . Then,

$$\Gamma = \{(w, x, t) : f(w, x) \geq t, f \in \tilde{\mathcal{F}}(\infty)\} = \{g(x)/G(x) \geq t\} \cap \{w > 0\} \cap \{w \leq x'\theta, \theta \in \mathbb{R}^d\}.$$

By Lemma 2.6.17 in [van der Vaart and Wellner \(1996\)](#)  $\tilde{\mathcal{F}}(\infty)$  is VC-subgraph with VC-index at most  $2d + 2$ . Therefore, by Haussler's VC bound for any probability measure  $Q$ ,  $r \geq 1$ , and  $0 < \eta < 1$

$$N\left(\eta, \tilde{\mathcal{F}}(\infty), L^r(Q)\right) \leq C(16e)^{2d+2} d \left(\frac{1}{\eta}\right)^{r(2d+1)}, \quad (\text{S.3.1})$$

where  $C > 0$  is a universal constant. For  $\delta > 0$  let

$$\sigma_n(G, \delta) = \sup_{f \in \mathcal{F}(r_n)} \|f\|_{L^2(\mathbb{P}_n)} \|G\|_{L^{2+\delta}(\mathbb{P}_n)}.$$

Without loss of generality we can assume that  $G > 1$  and hence  $\sigma_n(G, \delta) \geq \sup_{f \in \mathcal{F}(r_n)} \|f\|_{L^2(\mathbb{P}_n)}$ . For arbitrary  $f_1, f_2 \in \mathcal{F}(r_n)$ , the generalized Hölder inequality yields,

$$\begin{aligned} \|f_1 - f_2\|_{L^2(\mathbb{P}_n)}^2 \sigma_n^{-1}(G, \delta) &\leq \sup_{f \in \mathcal{F}(r_n)} \frac{2}{n} \sum_{i=1}^n \left| \frac{f_1(W_{ni}, X_{ni})}{G(X_{ni})} - \frac{f_2(W_{ni}, X_{ni})}{G(X_{ni})} \right| |f(W_{ni}, X_{ni}) G(X_{ni})| \sigma_n^{-1}(G, \delta) \\ &\leq 2 \|f_1/G - f_2/G\|_{L^{2+4/\delta}(\mathbb{P}_n)} \sup_{f \in \mathcal{F}(r_n)} \|f\|_{L^2(\mathbb{P}_n)} \|G\|_{L^{2+\delta}(\mathbb{P}_n)} \sigma_n^{-1}(G, \delta) \\ &= 2 \|f_1/G - f_2/G\|_{L^{2+4/\delta}(\mathbb{P}_n)}. \end{aligned} \quad (\text{S.3.2})$$

Eq. (S.3.2) implies that

$$N(\eta \sigma_n(G), \mathcal{F}(r_n), L^2(\mathbb{P}_n)) \leq N(\eta^2/2, \tilde{\mathcal{F}}(r_n), L^{2+4/\delta}(\mathbb{P}_n)) \leq N(\eta^2/2, \tilde{\mathcal{F}}(\infty), L^{2+4/\delta}(\mathbb{P}_n)). \quad (\text{S.3.3})$$

Thus, applying eq. (S.3.1) with  $Q = \mathbb{P}_n$  and  $r = 2 + 4/\delta$  to right side of eq. (S.3.3), yields

$$N(\eta \sigma_n(G), \mathcal{F}(r_n), L^2(\mathbb{P}_n)) \leq C(16e)^{2d+2} d \left(\frac{2}{\eta}\right)^{(2+4/\delta)(2d+1)}. \quad (\text{S.3.4})$$

**Step 2. Combinatorial bounds.** Let  $\varepsilon = (\varepsilon_1, \dots, \varepsilon_n)$  be a vector of i.i.d Rademacher random variables independent of  $(W_{n1}, X_{n1}), \dots, (W_{nn}, X_{nn})$ . By Dudley's entropy inequality (e.g. [van der Vaart and Wellner, 1996](#), Corollary 2.2.8) inequality (S.3.4), a change of variable, two applications of the Cauchy-Schwarz inequality and one of Jensen's inequality,

$$\begin{aligned} &\mathbb{E} \left[ \sup_{f \in \mathcal{F}(r_n)} \frac{1}{n} \sum_{i=1}^n (f(W_{ni}, X_{ni}) - \mathbb{E}f(W_{ni}, X_{ni})) \right] \\ &\leq 2 \mathbb{E} \left[ \sup_{f \in \mathcal{F}(r_n)} \frac{1}{n} \sum_{i=1}^n \varepsilon_i f(W_{ni}, X_{ni}) \right] \end{aligned}$$

$$\begin{aligned}
&\leq \frac{C_1}{n^{1/2}} \mathbb{E} \left[ \int_0^{\sigma_n(G, \delta)} \left( \log N(\eta, \mathcal{F}(r_n), L^2(\mathbb{P}_n)) \right)^{1/2} d\eta \right] \\
&\leq C_1 \left( \frac{d}{n} \right)^{1/2} \mathbb{E} [\sigma_n(G, \delta)] \int_0^1 (\log(1/\eta))^{1/2} d\eta \\
&\leq C_1 \left( \frac{d}{n} \right)^{1/2} \mathbb{E} \left[ \sup_{f \in \mathcal{F}(r_n)} \frac{1}{n} \sum_{i=1}^n f^2(W_{ni}, X_{ni}) \right]^{1/2} \mathbb{E} \left[ \frac{1}{n} \sum_{i=1}^n G^{2+\delta}(X_{ni}) \right]^{1/(2+\delta)}, \tag{S.3.5}
\end{aligned}$$

where  $C_1 > 0$  is an absolute constant that may change from line to line. Analogously,

$$\begin{aligned}
&\mathbb{E} \left[ \sup_{f \in \mathcal{F}(r_n)} \frac{1}{n} \sum_{i=1}^n (f^2(W_{ni}, X_{ni}) - \mathbb{E} f^2(W_{ni}, X_{ni})) \right] \\
&\leq C_2 \left( \frac{d}{n} \right)^{1/2} \mathbb{E} \left[ \sup_{f \in \mathcal{F}(r_n)} \frac{1}{n} \sum_{i=1}^n f^4(W_{ni}, X_{ni}) \right]^{1/2} \mathbb{E} \left[ \frac{1}{n} \sum_{i=1}^n G^{4+2\delta}(X_{ni}) \right]^{1/(2+\delta)}, \tag{S.3.6}
\end{aligned}$$

where  $C_2 > 0$  is an absolute constant.

**Step 3. Moment bounds.** By the boundedness of the conditional density of  $W_{ni}|X_{ni}$ ,

$$\begin{aligned}
&\mathbb{E} \left[ \sup_{f \in \mathcal{F}(r_n)} \frac{1}{n} \sum_{i=1}^n f^2(W_{ni}, X_{ni}) \right] \\
&\leq \mathbb{E} \left[ \sup_{f \in \mathcal{F}(r_n)} \frac{1}{n} \sum_{i=1}^n f^2(W_{ni}, X_{ni}) - \mathbb{E} [f^2(W_{ni}, X_{ni})] \right] \sup_{f \in \mathcal{F}(r_n)} \mathbb{E} \left[ \frac{1}{n} \sum_{i=1}^n f^2(W_{ni}, X_{ni}) \right] \\
&\leq \mathbb{E} \left[ \sup_{f \in \mathcal{F}(r_n)} \frac{1}{n} \sum_{i=1}^n f^2(W_{ni}, X_{ni}) - \mathbb{E} [f^2(W_{ni}, X_{ni})] \right] + r_n \left( \sup_{\|u\|_2=1} \mathbb{E} \left[ \frac{F_+}{n} \sum_{i=1}^n (X'_{ni} u) G^2(X_{ni}) \right] \right). \tag{S.3.7}
\end{aligned}$$

Since  $0 \leq f \leq 1 \leq G$ ,

$$\mathbb{E} \left[ \sup_{f \in \tilde{\mathcal{F}}(r_n)} \frac{1}{n} \sum_{i=1}^n f^4(W_{ni}, X_{ni}) \right] \leq \mathbb{E} [G^4(X_{n1})]. \tag{S.3.8}$$

**Step 4. Conclusion.** We now combine the combinatorial and moment bounds.

$$\begin{aligned}
&\mathbb{E} \left[ \sup_{f \in \mathcal{F}} \frac{1}{n} \sum_{i=1}^n (f(W_{ni}, X_{ni}) - \mathbb{E} f(W_{ni}, X_{ni})) \right] \\
&\leq C_1 \left( \frac{d}{n} \right)^{1/2} \mathbb{E} \left[ \sup_{f \in \mathcal{F}(r_n)} \frac{1}{n} \sum_{i=1}^n f^2(W_{ni}, X_{ni}) \right]^{1/2} \mathbb{E} \left[ \frac{1}{n} \sum_{i=1}^n G^{2+\delta}(X_{ni}) \right]^{1/(2+\delta)} \\
&\leq C_1 \left( \frac{d}{n} \right)^{1/2} \left| \mathbb{E} \left[ \sup_{f \in \mathcal{F}(r_n)} \frac{1}{n} \sum_{i=1}^n f^2(W_{ni}, X_{ni}) - \mathbb{E} [f^2(W_{ni}, X_{ni})] \right] \right|^{1/2} \mathbb{E} \left[ \frac{1}{n} \sum_{i=1}^n G^{2+\delta}(X_{ni}) \right]^{1/(2+\delta)}
\end{aligned}$$

$$\begin{aligned}
& + C_1 \left( \frac{d}{n} \right)^{1/2} r_n^{1/2} \left( \sup_{\|u\|_2=1} \mathbb{E} \left[ \frac{F_+}{n} \sum_{i=1}^n (X'_{ni} u) G^2(X_{ni}) \right] \right)^{1/2} \mathbb{E} \left[ \frac{1}{n} \sum_{i=1}^n G^{2+\delta}(X_{ni}) \right]^{1/(2+\delta)} \\
& \leq C_1 C_2^{1/2} \left( \frac{d}{n} \right)^{3/4} \mathbb{E} \left[ \sup_{f \in \mathcal{F}(r_n)} \frac{1}{n} \sum_{i=1}^n f^4(W_{ni}, X_{ni}) \right]^{1/4} \mathbb{E} \left[ \frac{1}{n} \sum_{i=1}^n G^{4+2\delta}(X_{ni}) \right]^{1/(4+2\delta)} \mathbb{E} \left[ \frac{1}{n} \sum_{i=1}^n G^{2+\delta}(X_{ni}) \right]^{1/(2+\delta)} \\
& \quad + C_1 \left( \frac{d}{n} \right)^{1/2} r_n^{1/2} \left( \sup_{\|u\|_2=1} \mathbb{E} \left[ \frac{F_+}{n} \sum_{i=1}^n (X'_{ni} u) G^2(X_{ni}) \right] \right)^{1/2} \mathbb{E} \left[ \frac{1}{n} \sum_{i=1}^n G^{2+\delta}(X_{ni}) \right]^{1/(2+\delta)} \\
& \leq C_1 C_2^{1/2} \left( \frac{d}{n} \right)^{3/4} \mathbb{E} [G^4(X_{n1})]^{1/4} \mathbb{E} [G^{4+2\delta}(X_{n1})]^{1/(4+2\delta)} \mathbb{E} [G^{2+\delta}(X_{n1})]^{1/(2+\delta)} \\
& \quad + C_1 \left( \frac{d}{n} \right)^{1/2} r_n^{1/2} F_+^{1/2} \left( \sup_{\|u\|_2=1} \mathbb{E} [(X'_{n1} u) G^2(X_{n1})] \right)^{1/2} \mathbb{E} [G^{2+\delta}(X_{n1})]^{1/(2+\delta)}, \tag{S.3.9}
\end{aligned}$$

where the first inequality follows from eq. (S.3.5), the second from eq. (S.3.7) and the third from eq. (S.3.6). The fourth inequality holds since  $X_{ni}$  are identically distributed.  $\square$

**Lemma S.3.3.** *Let  $\{X_{ni}, i = 1, \dots, n\}$  be triangular array of row-wise i.i.d.  $\mathbb{R}^d$ -valued random vectors. Let  $\max_{\|u\|_2=1} \mathbb{E} [(X'_{n1} u)^2] \leq \lambda_+$ . Suppose that there exists  $p \geq 1$  and an absolute constant  $\mu_{4p} < \infty$ , independent of  $d$ , such that  $\max_{1 \leq k \leq d} \mathbb{E} [(X_{n1}^{(k)})^{4p}] \leq \mu_{4p}$ . Then,*

$$\sup_{\|v\|_2=1} \left( \mathbb{E} \left[ \frac{1}{n} \sum_{i=1}^n |X'_{ni} v|^{2p} \right] \right)^{1/(2p)} \leq 2^{2+1/(2p)} K^{1/2} p^{1/2} \mu_{4p}^{1/(2p)} + \lambda_+^{1/2},$$

where  $K = 1/(e - \sqrt{e})$ .

*Proof.* Let  $\varepsilon = (\varepsilon_1, \dots, \varepsilon_d)$  be a vector of i.i.d. Rademacher variables independent of  $X_n = (X_n^{(1)}, \dots, X_n^{(d)})$ . Let  $K = 1/(e - \sqrt{e})$ ,  $p \geq 1$ , and  $\|v\|_2 = 1$ ,  $v \in \mathbb{R}^d$ . Then,

$$\begin{aligned}
\left( \mathbb{E} \left[ \frac{1}{n} \sum_{i=1}^n |X'_{ni} v|^{2p} \right] \right)^{1/(2p)} & \leq \left( \mathbb{E} \left[ \left| \sum_{k=1}^d X_{n1}^{(k)} v_k - \mathbb{E} [X_{n1}^{(k)} v_k] \right|^{2p} \right] \right)^{1/(2p)} + |\mathbb{E} [X'_n v]| \\
& \leq 2 \left( \mathbb{E} \left[ \left| \sum_{k=1}^d \varepsilon_k X_{n1}^{(k)} v_k \right|^{2p} \right] \right)^{1/(2p)} + |\mathbb{E} [(X'_n v)^2]|^{1/2} \\
& \leq 2^{2+1/(2p)} K^{1/2} p^{1/2} \left( \mathbb{E} \left[ \left( \sum_{k=1}^d (X_{n1}^{(k)} v_k)^2 \right)^{2p} \right] \right)^{1/(2p)} + \lambda_+^{1/2} \\
& \leq 2^{2+1/(2p)} K^{1/2} p^{1/2} \sum_{k=1}^d \left( \mathbb{E} [(X_{n1}^{(k)} v_k)^{4p}] \right)^{1/(2p)} + \lambda_+^{1/2} \\
& = 2^{2+1/(2p)} K^{1/2} p^{1/2} \sum_{k=1}^d \mu_{4p}^{1/(2p)} v_k^2 + \lambda_+^{1/2}
\end{aligned}$$

$$\leq 2^{2+1/(2p)} K^{1/2} p^{1/2} \mu_{4p}^{1/(2p)} + \lambda_+^{1/2}, \quad (\text{S.3.10})$$

where the second inequality follows from Jensen's and the symmetrization inequality for conditional Rademacher averages, the third from Khinchine's inequality for conditional Rademacher averages, the fourth from Minkowski's integral inequality, and the remaining inequalities from elementary calculations. Note that eq. (S.3.10) is independent of  $n$ ,  $d$ , and  $v$ . This concludes the proof.  $\square$

The next lemma provides an almost sure bound on the centered quantile regression score.

**Lemma S.3.4.** *Suppose that Assumptions (A1) – (A6) hold. There exists an absolute constants  $N_0, c_0 > 0$  such that for any  $r_n > 0$  and all  $n > N_0$ ,*

$$\begin{aligned} \sup_{S \in M} \sup_{\|\delta\|_2 = r_n} \left\| \frac{1}{n} \sum_{i=1}^n -\varphi_\tau(e_{ni,S}^\tau - Z'_{ni,S}\delta)Z_{ni,S} + \varphi_\tau(e_{ni,S}^\tau)Z_{ni,S} + \mathbb{E}_{\mathcal{D}_n} [\varphi_\tau(e_{ni,S}^\tau - Z'_{ni,S}\delta)Z_{ni,S} - \varphi_\tau(e_{ni,S}^\tau)Z_{ni,S}] \right\|_2 \\ \leq c_0 r_n^{1/2} \left( \frac{m \log |M|}{n} \right)^{1/2} + c_0 \left( \frac{m \log |M| \log \log n}{n} \right)^{3/4} \quad a.s. \end{aligned}$$

*Proof.* The Lemma can be proved as Lemma 3.3 in He and Shao (2000) but with Lemma 3.1 (He and Shao, 2000) replaced by Lemma S.3.1.  $\square$

The following lemma provides an almost sure bound on the (un-centered) quantile regression score.

**Lemma S.3.5.** *Suppose that Assumptions (A1) – (A6) hold. There exists an absolute constants  $N_1, c_1 > 0$  such that for all  $n > N_1$ ,*

$$\sup_{S \in M} \left\| \frac{1}{n} \sum_{i=1}^n \varphi_\tau(e_{ni,S}^\tau)Z_{ni,S} \right\|_2 \leq c_1 \left( \frac{m + \log |M| + \log \log n}{n} \right)^{1/2} \quad a.s.$$

*Proof.* We combine Lemma S.3.1 with upper bounds on the expected value of the supremum of the empirical process under consideration and the corresponding mixed uniform variance.

**Step 1. Decomposition.** We upper bound the process by two empirical processes and then analyze those processes separately:

$$\begin{aligned} \sup_{S \in M} \left\| \frac{1}{n} \sum_{i=1}^n \varphi_\tau(e_{ni,S}^\tau)Z_{ni,S} \right\|_2 \\ \leq \sup_{S \in M} \sup_{\|u_S\|_2=1} \frac{1}{n} \sum_{i=1}^n \left( Z'_{ni,S}u_S - \mathbb{E}_{\mathcal{D}_n} [Z'_{ni,S}u_S] \right) \\ + \sup_{S \in M} \sup_{\|u_S\|_2=1} \frac{1}{n} \sum_{i=1}^n \left( 1\{e_{ni,S}^\tau \leq 0\}Z'_{ni,S}u_S - \mathbb{E}_{\mathcal{D}_n} [1\{e_{ni,S}^\tau \leq 0\}Z'_{ni,S}u_S] \right). \end{aligned}$$

**Step 2. Almost sure bound on the first term.** For fixed  $S \in M$  let  $\mathcal{N}_S$  be a  $\frac{1}{2}$ -net of the

unit sphere in  $\mathbb{R}^{|S|}$ . Then,

$$\sup_{\|u_S\|_2=1} \frac{1}{n} \sum_{i=1}^n \left( Z'_{ni,S} u_S - \mathbb{E}_{\mathcal{D}_n} [Z'_{ni,S} u_S] \right) \leq \max_{v \in \mathcal{N}_S} \frac{2}{n} \sum_{i=1}^n \left( Z'_{ni,S} v - \mathbb{E}_{\mathcal{D}_n} [Z'_{ni,S} v] \right).$$

Let  $\mathcal{D}_n^0$  be an independent copy of  $\mathcal{D}_n$ . For  $v \in \mathcal{N}_S$  define

$$W_n(S, v) = \mathbb{E}_{\mathcal{D}_n^0} \left[ \frac{1}{n} \sum_{i=1}^n \left( Z'_{ni,S} v - Z_{ni,S}^0 v \right)^2 \middle| \mathcal{D}_n \right].$$

By the Hartman-Wintner law of iterated logarithm there exists an  $N_S > 0$  such that for all  $n > N_S$  and for all  $v \in \mathcal{N}_S$ ,

$$\begin{aligned} W_n(S, v) &\leq \frac{2}{n} \sum_{i=1}^n (v' Z_{ni,S})^2 + \mathbb{E}_{\mathcal{D}_n} \left[ \frac{2}{n} \sum_{i=1}^n (v' Z_{ni,S})^2 \right] \\ &\leq \frac{2}{n} \sum_{i=1}^n \left( (v' Z_{ni,S})^2 - \mathbb{E}_{\mathcal{D}_n} [(v' Z_{ni,S})^2] \right) + \frac{4}{n} \mathbb{E}_{\mathcal{D}_n} [(v' Z_{n1,S})^2] \\ &\leq \frac{2}{n} \mathbb{E}_{\mathcal{D}_n} [(v' Z_{n1,S})^4]^{1/2} \left( \frac{\log \log n}{n} \right)^{1/2} + 4 \frac{\lambda_+}{n} \\ &\leq c_1/n, \end{aligned}$$

where  $c_1 > 0$  is a constant independent of  $n$  and  $S$ .

Thus, by the union bound and Lemma S.3.1, for all  $n > N_0 \equiv \max_{S \in M} N_S$  and for any  $t > 0$ ,

$$\begin{aligned} \mathbb{P} \left( \sup_{S \in M} \sup_{\|u_S\|_2=1} \frac{1}{n} \sum_{i=1}^n \left( Z'_{ni,S} u_S - \mathbb{E}_{\mathcal{D}_n} [Z'_{ni,S} u_S] \right) \geq 4c_1 \left( \frac{t + 2m \log 5 + \log |M|}{n} \right)^{1/2} \right) \\ \leq 4e \sum_{S \in M} |\mathcal{N}_S| e^{-m \log 5 - \log |M| - t/2} \\ \leq 4e e^{-t/2}. \end{aligned}$$

Standard arguments now guarantee that there exists a universal constant  $c_1 > 0$  and  $N'_0 \geq N_0$  such that for all  $n > N'_0$ ,

$$\sup_{S \in M} \sup_{\|u_S\|_2=1} \frac{1}{n} \sum_{i=1}^n \left( Z'_{ni,S} u_S - \mathbb{E}_{\mathcal{D}_n} [Z'_{ni,S} u_S] \right) \leq c_1 \left( \frac{m + \log |M| + \log \log n}{n} \right)^{1/2}. \quad (\text{S.3.11})$$

**Step 3. Almost sure bound on the second term.** Follows in the same way as the bound on the first term.  $\square$

The final lemma is a strengthened version of Theorems 2.1 and 2.2 in [He and Shao \(2000\)](#) in the special case of quantile regressions.

**Lemma S.3.6.** *Suppose that Assumptions (A1) – (A6) hold. Then, there exists a universal constants  $N_2, c_2, c_3 > 0$  such that for all  $n > N_2$ ,*

$$\hat{\theta}_{n,S}^\tau = \theta_{n,S}^\tau + \left( \mathbb{E} [f_{Y_n|X_n}(Z'_{n1,S}\theta_{n,S}^\tau|X_{n1})Z_{n1,S}Z'_{n1,S}] \right)^{-1} \frac{1}{n} \sum_{i=1}^n \varphi_\tau(e_{n,S}^\tau) Z_{ni,S} + r_{n,S}^\tau,$$

and

$$\sup_{S \in M} \|r_{n,S}^\tau\|_2 \leq \frac{c_2}{\lambda_n^2} \left( \frac{m \log |M| \log \log n}{n} \right)^{1/4} \left( \frac{m \log |M| + \log \log n}{n} \right)^{1/2} \quad a.s.,$$

and

$$\sup_{S \in M} \|\hat{\theta}_{n,S}^\tau - \theta_{n,S}^\tau\|_2 \leq \frac{c_3}{\lambda_n} \left( \frac{m \log |M| \log \log n}{n} \right)^{1/2} \quad a.s.$$

*Proof.* The claims follow from Lemma S.3.5 and steps analogous to those in the proofs of the corresponding theorems in He and Shao (2000) but with Lemma 3.3 (He and Shao, 2000) replaced by Lemma S.3.4.  $\square$

#### S.4. Numerical evidence

In this section we provide further numerical evidence for the DGPs 2–4 from Section 5 in the main paper. The interpretations given in Section 5 apply to below plots as well. Qualitatively, the conclusion for DGPs 2–4 are the same for DGP1. However, the variations are sometimes higher in the results because DGP 2–4 involve more complex settings.

#### References

- Akaike, H., 1992. Information theory and an extension of the maximum likelihood principle, in: Kotz, S., Johnson, N.L. (Eds.), Breakthroughs in Statistics: Foundations and Basic Theory, Springer-Verlag, New York. pp. 610–624. doi:[10.1007/978-1-4612-0919-5\\_38](https://doi.org/10.1007/978-1-4612-0919-5_38).
- Akaike, H., 1998. Statistical predictor identification, in: Akaike, H., Parzen, E., Tanabe, K., Kitagawa, G. (Eds.), Selected Papers of Hirotugu Akaike, Springer-Verlag, New York. pp. 137–151. doi:[10.1007/978-1-4612-1694-0\\_1](https://doi.org/10.1007/978-1-4612-1694-0_1).
- Angrist, J., Chernozhukov, V., Fernández-Val, I., 2006. Quantile regression under misspecification, with an application to the U.S. wage structure. *Econometrica* 74, 539–563. doi:[10.1111/j.1468-0262.2006.00671.x](https://doi.org/10.1111/j.1468-0262.2006.00671.x).
- He, X., Shao, Q.M., 2000. On parameters of increasing dimensions. *Journal of Multivariate Analysis* 73, 120–135. doi:[10.1006/jmva.1999.1873](https://doi.org/10.1006/jmva.1999.1873).

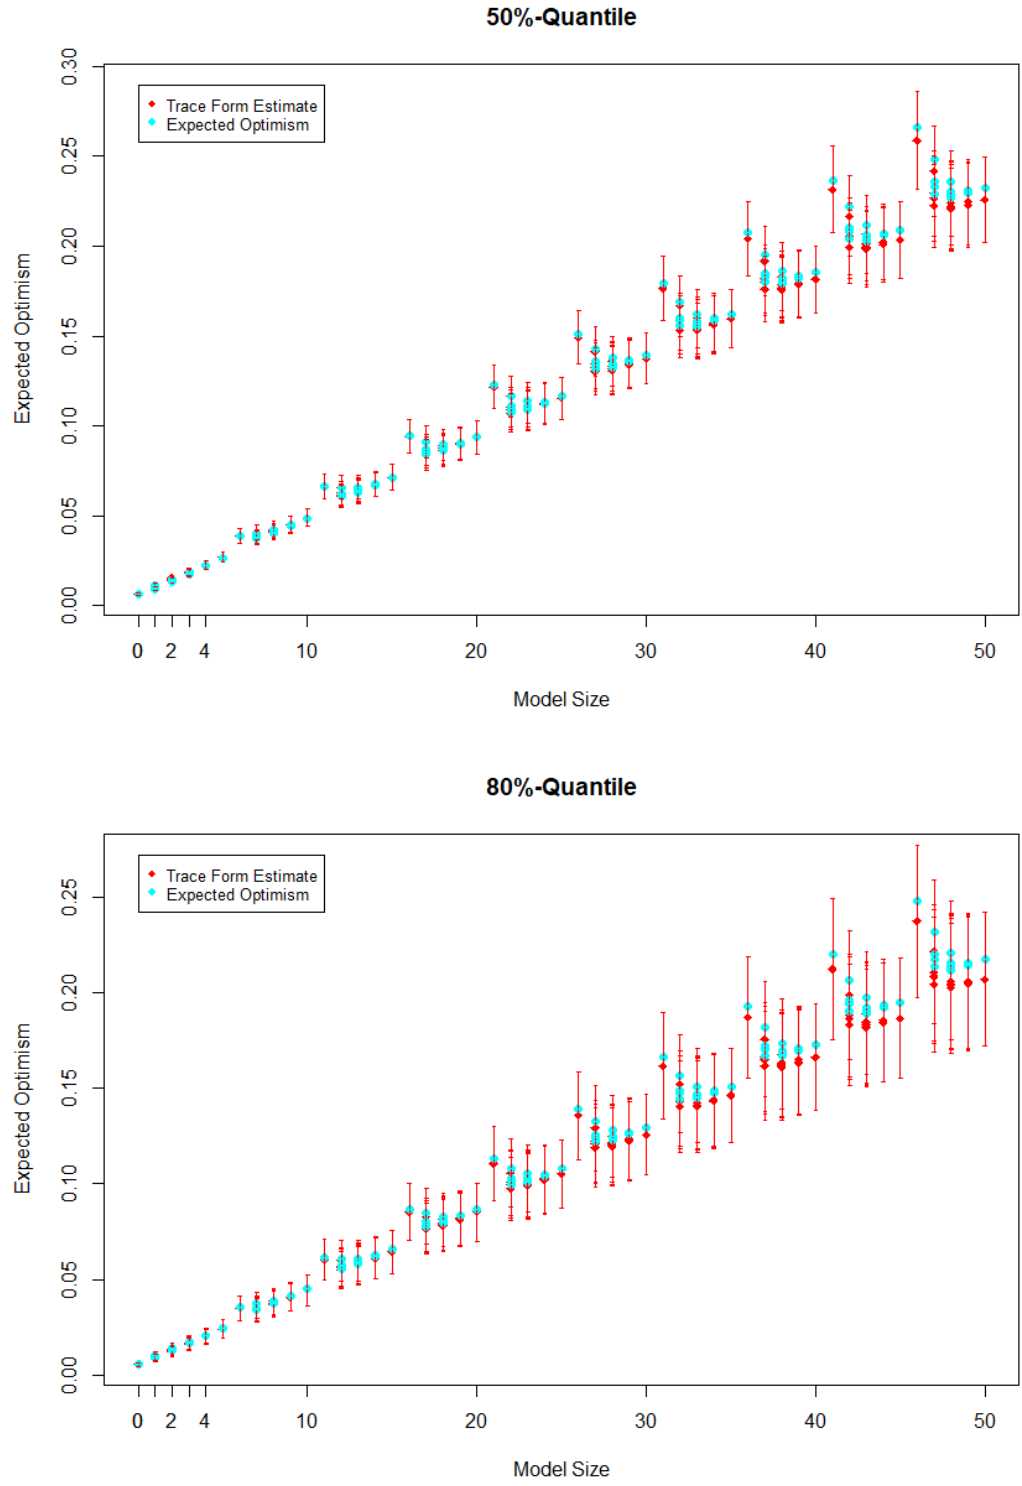

Figure 1: Red: estimates of the trace form and standard errors. Blue: expected optimism. Top: DGP2 with  $\tau = 0.5$ . Bottom: DGP2 with  $\tau = 0.8$ .

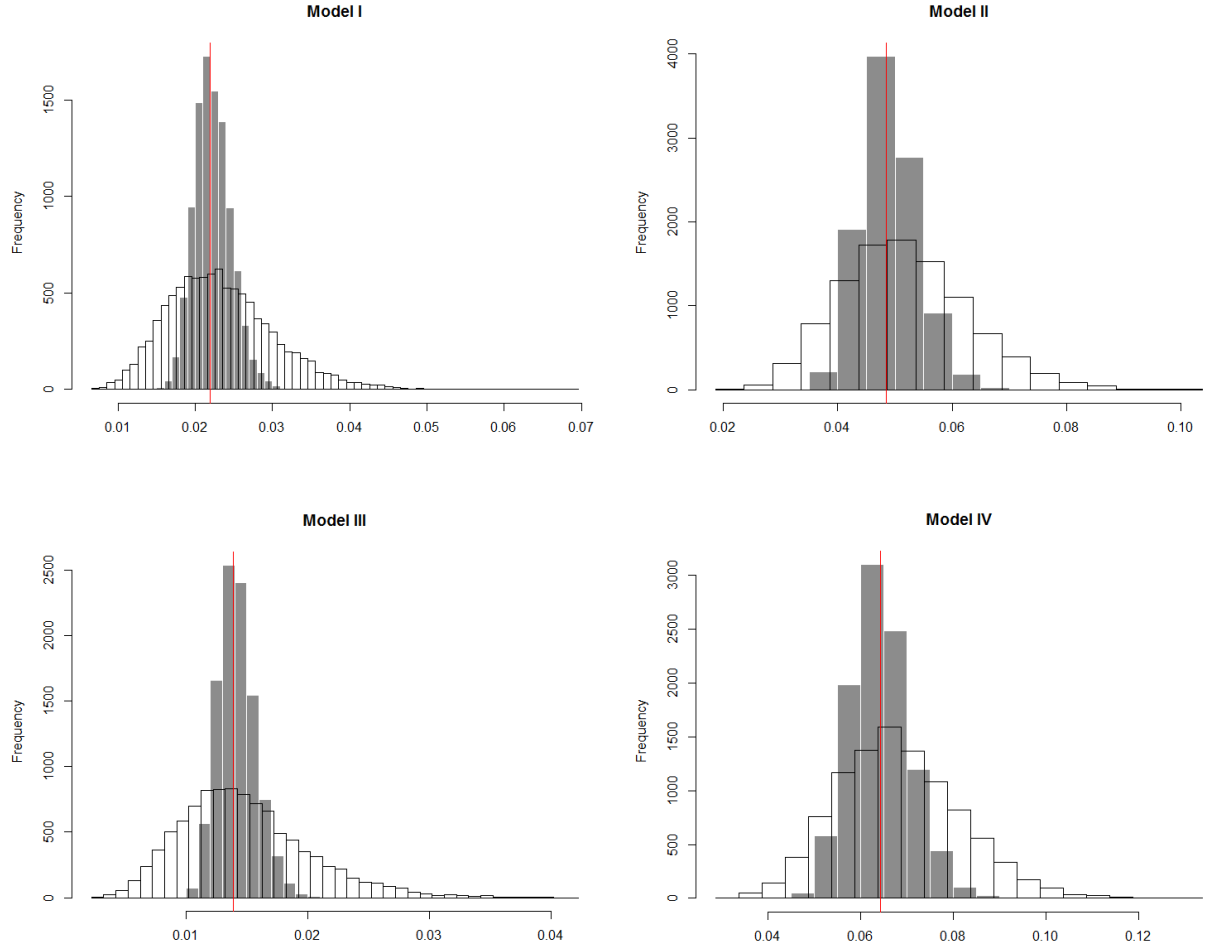

Figure 2: Histograms of the 10-fold CV estimate of the expected optimism and the trace form estimate for DGP2 and  $\tau = 0.5$ . Red line: expected optimism. White histogram: 10-fold CV. Model I: correct model (with predictors 1 to 4), Model II: an over-fitted model (with predictors 1 to 10), Model III: an under-fitted model (with predictors 1 to 2) and Model IV that comprises the relevant predictors 1 and 2 and the irrelevant predictors 5 to 15.

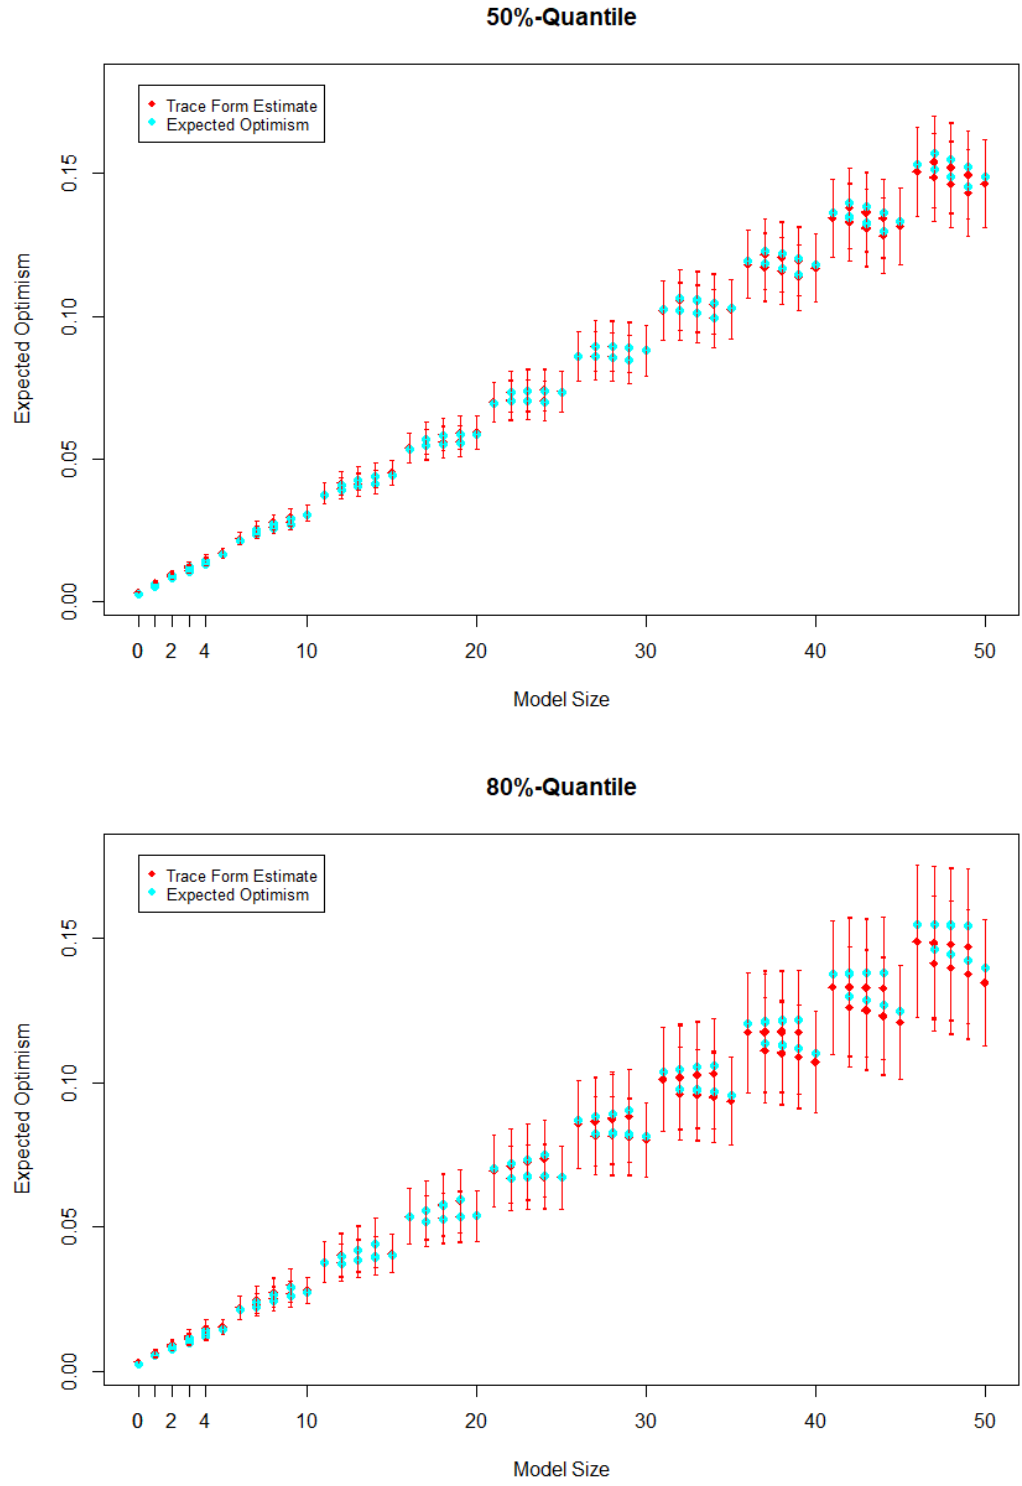

Figure 3: Red: estimates of the trace form and standard errors. Blue: expected optimism. Top: DGP3 with  $\tau = 0.5$ . Bottom: DGP3 with  $\tau = 0.8$ .

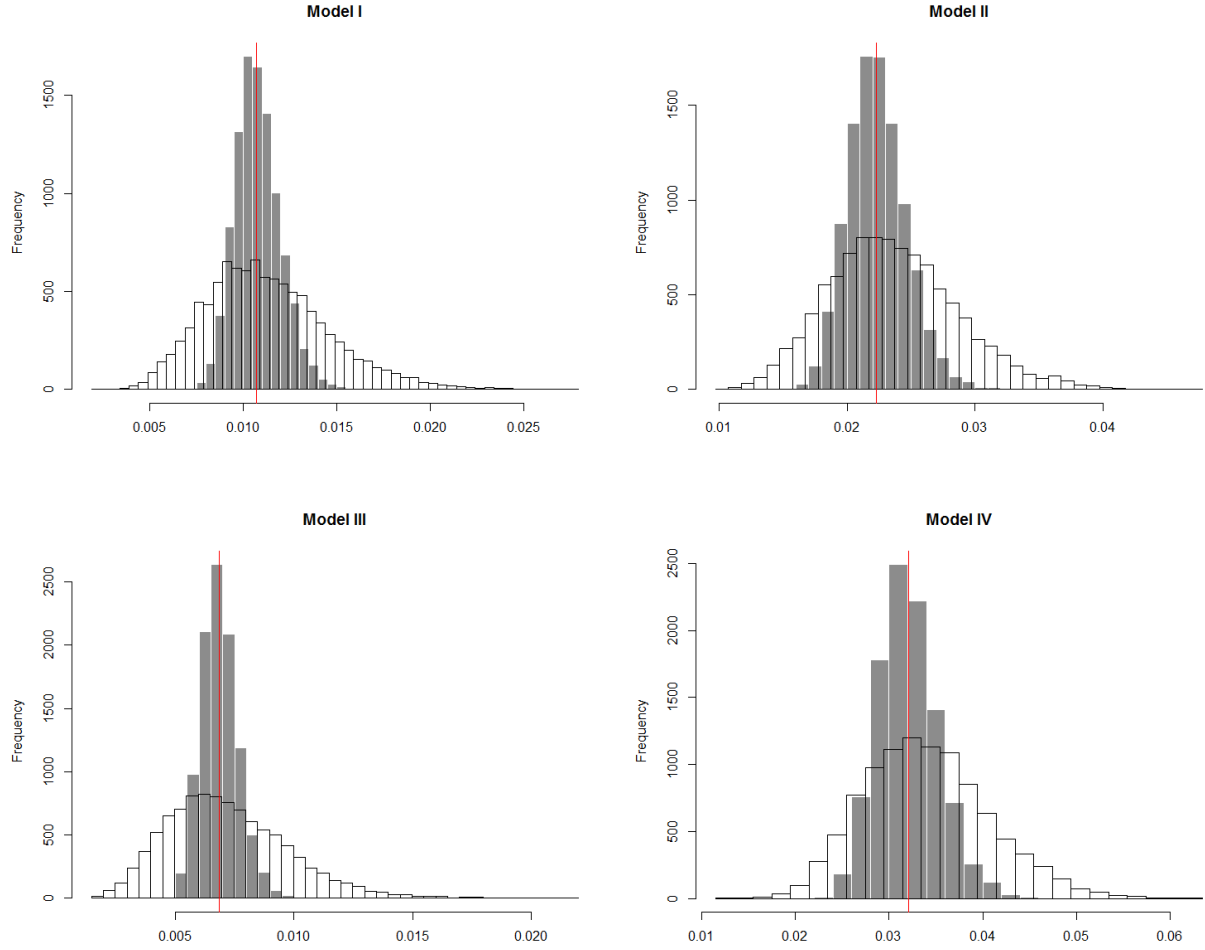

Figure 4: Histograms of the 10-fold CV estimate of the expected optimism and the trace form estimate for DGP3 and  $\tau = 0.5$ . Red line: expected optimism. White histogram: 10-fold CV. Model I: correct model (with predictors 1 to 4), Model II: an over-fitted model (with predictors 1 to 10), Model III: an under-fitted model (with predictors 1 to 2) and Model IV that comprises the relevant predictors 1 and 2 and the irrelevant predictors 5 to 15.

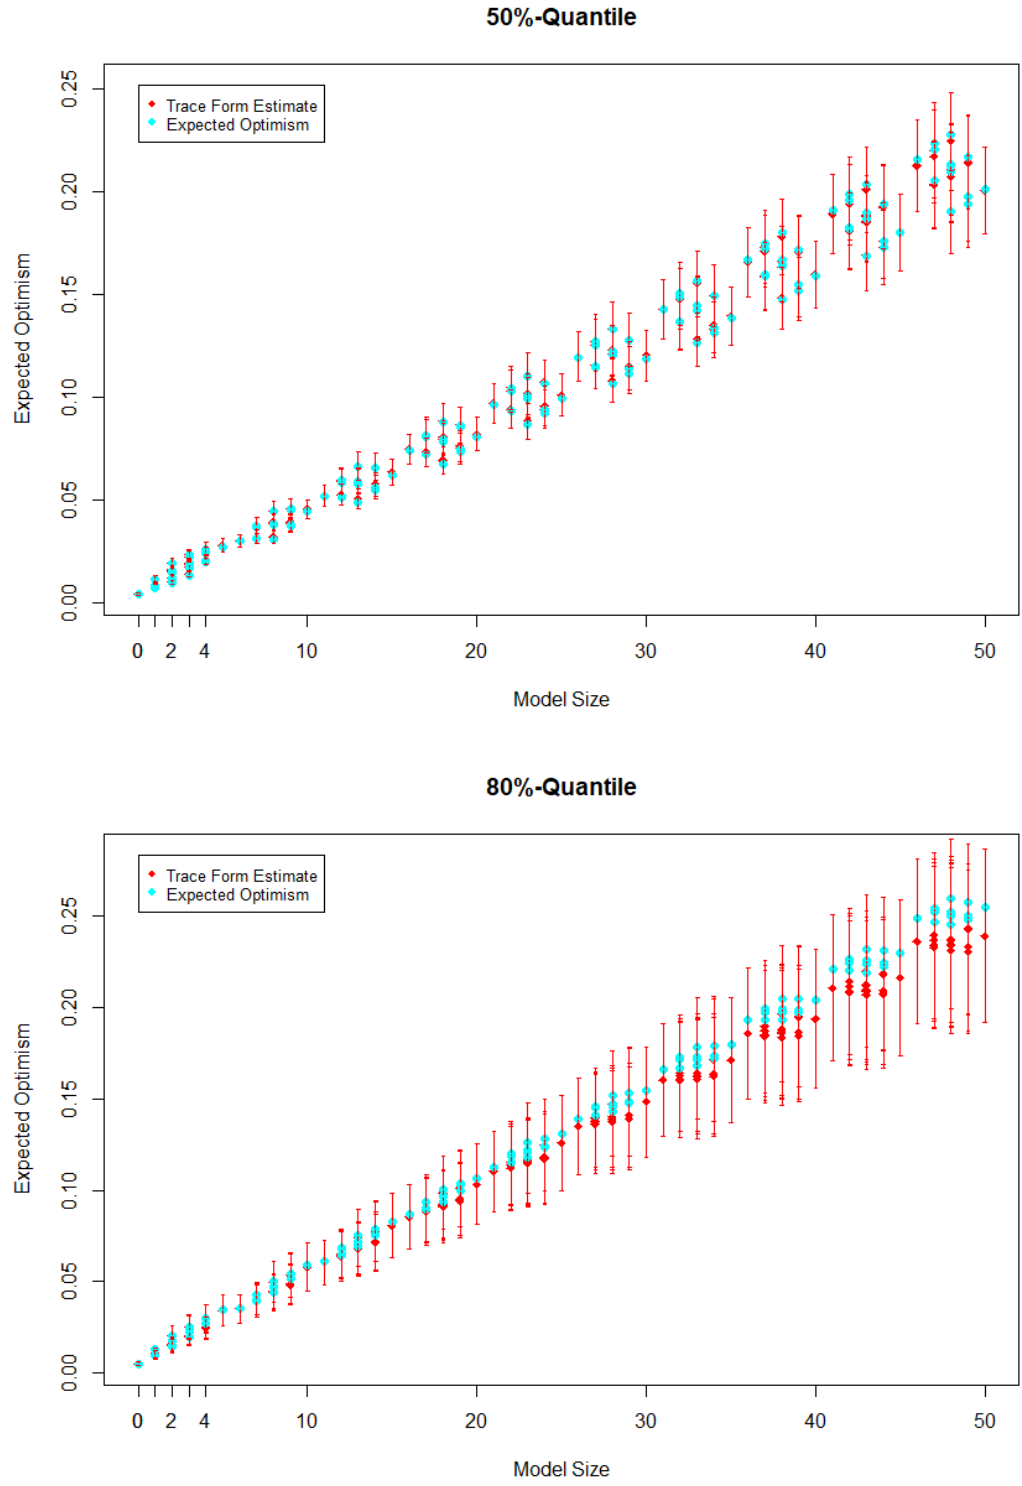

Figure 5: Red: estimates of the trace form and standard errors. Blue: expected optimism. Top: DGP4 with  $\tau = 0.5$ . Bottom: DGP4 with  $\tau = 0.8$ .

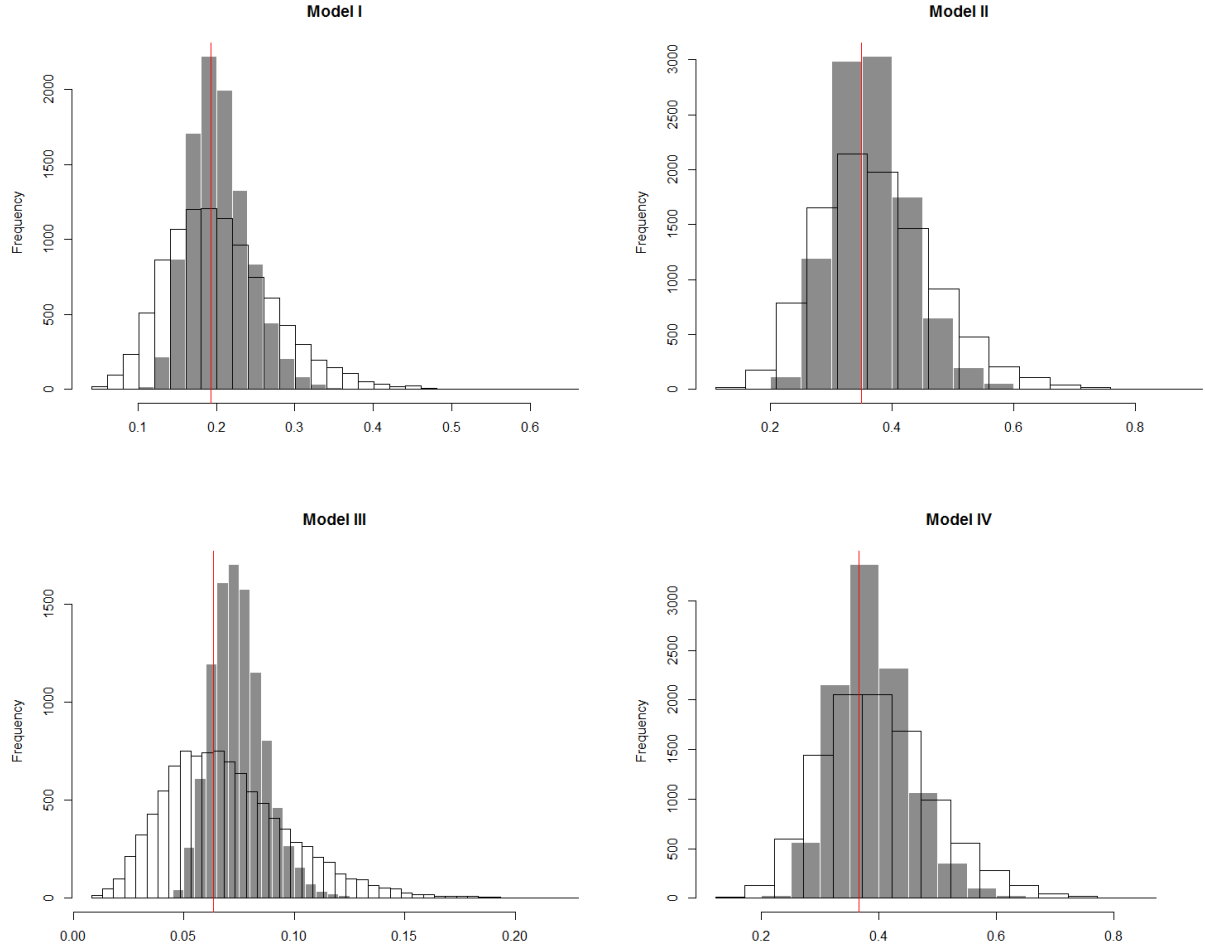

Figure 6: Histograms of the 10-fold CV estimate of the expected optimism and the trace form estimate for DGP4 and  $\tau = 0.5$ . Red line: expected optimism. White histogram: 10-fold CV. Model I: correct model (with predictors 1 to 4), Model II: an over-fitted model (with predictors 1 to 10), Model III: an under-fitted model (with predictors 1 to 2) and Model IV that comprises the relevant predictors 1 and 2 and the irrelevant predictors 5 to 15.

- Lv, J., Liu, J.S., 2014. Model selection principles in misspecified models. *Journal of the Royal Statistical Society: Series B (Statistical Methodology)* 76, 141–167. doi:[10.1111/rssb.12023](https://doi.org/10.1111/rssb.12023).
- Panchenko, D., 2003. Symmetrization approach to concentration inequalities for empirical processes. *The Annals of Probability* 31, 2068–2081. doi:[10.1214/aop/1068646378](https://doi.org/10.1214/aop/1068646378).
- van der Vaart, A.W., Wellner, J., 1996. *Weak Convergence and Empirical Processes: With Applications to Statistics*. Springer Series in Statistics, Springer-Verlag, New York.
